# Supplementary material for: Variational inference for sparse network reconstruction from count data
Source: arXiv:1806.03120 source file (2018-06-08)
Supplement: Supplementary file 1 [file VEM-PLNnetwork-appendix.tex]

\section{Appendix} \label{sec:appendix}

%%%%%%%%%%%%%%%%%%%%%%%%%%%%%%%%%%%%%%%%%%%%%%%%%%%%%%%%%%%%%%%%%%%%%%%%%%%%%%%
\subsection{Gradients}
%%%%%%%%%%%%%%%%%%%%%%%%%%%%%%%%%%%%%%%%%%%%%%%%%%%%%%%%%%%%%%%%%%%%%%%%%%%%%%%
